# Supplementary material for: Tensor hypercontraction for fully self-consistent imaginary-time GF2 and GWSOX methods: theory, implementation, and role of the Green's function second-order exchange for intermolecular interactions
Source: arXiv:2404.17744 source file (2024-04-27)
Supplement: Supplementary file 1 [file SI.pdf]

# Tensor hypercontraction for fully self-consistent imaginary-time GF2 and GWSOX methods: theory, implementation, and role of the Green's function second-order exchange for intermolecular interactions

Pavel Pokhilko,[1] Chia-Nan Yeh,[2] Miguel A. Morales,[2] and Dominika Zgid[1,3]

[1]*Department of Chemistry, University of Michigan, Ann Arbor, Michigan 48109, USA*

[2]*Center for Computational Quantum Physics, Flatiron Institute, New York, New York 10010, USA*

[3]*Department of Physics, University of Michigan, Ann Arbor, Michigan 48109, USA*

TABLE S1: Interaction energies (kcal/mol) of selected systems from the S22 set computed with MP2 and fcMP2 and aug-cc-pVTZ with and without counterpoise correction. The all-electron MP2 calculations are computed using even-tempered auxiliary basis with beta=1.5 unless noted separately. The fcMP2 estimates are from Ref.[1].

| | | w/o CP | | w CP | |
|---|---|---|---|---|---|
| # | H-bonded | MP2 | fcMP2 | MP2 | fcMP2 |
| 1 | $(NH_3)_2$ | -3.44 | -3.24 | -3.00 | -2.99 |
| 2 | $(H_2O)_2$ | -5.63 | -5.16 | -4.71 | -4.69 |
| 3 | Formic acid dimer | -20.46 | -19.07 | -17.62 | -17.55 |
| 4 | Formamide dimer | -17.90 | -16.28 | -15.08 | -15.03 |
| | Dispersion dominated | MP2 | fcMP2 | MP2 | fcMP2 |
| 8 | $(CH_4)_2$ | -0.86 | -0.6 | -0.46 | -0.46 |
| 9 | Ethene dimer | -2.33 | -1.87 | -1.47 | -1.46 |
| 10 | Benzene-$CH_4$ [a] | -3.51 | -2.41 | -1.72 | -1.71 |
| | Mixed | MP2 | fcMP2 | MP2 | fcMP2 |
| 16 | Ethene-Ethine | -2.84 | -1.99 | -1.59 | -1.58 |
| 17 | Benzene-$H_2O$ [a] | -5.15 | -4.16 | -3.37 | -3.35 |
| 18 | Benzene-$NH_3$ [a] | -4.27 | -3.25 | -2.53 | -2.52 |
| 19 | Benzene-HCN [a] | -8.08 | -6.04 | -4.95 | -4.92 |

[a] For these systems due to nearly linear dependence of auxiliary functions we used even-tempered auxiliary basis with beta=1.6.

TABLE S2: Counterpoise-corrected interaction energies (kcal/mol) of selected systems from the S22 set computed with scGF2dir and scGF2 and aug-cc-pVTZ. Some scGF2dir calculations were not converging due to numerical difficulties in finding chemical potential. The fcCCSD estimates are from Ref.[1, 2].

| # | H-bonded | THC-scGF2dir | THC-scGF2 | fcCCSD |
|---|---|---|---|---|
| 1 | $(NH_3)_2$ | -4.25 | -3.82 | -2.733 |
| 2 | $(H_2O)_2$ | -5.73 | -5.60 | -4.496 |
| 3 | Formic acid dimer | -26.29 | -23.30 | -16.970 |
| 4 | Formamide dimer | -23.41 | -20.02 | -14.559 |
| | Dispersion dominated | THC-scGF2dir | THC-scGF2 | fcCCSD |
| 8 | $(CH_4)_2$ | -1.31 | -0.93 | -0.380 |
| 9 | Ethene dimer | -4.74 | -3.19 | -1.035 |
| 10 | Benzene-$CH_4$ | — | -4.17 | -0.960 |
| | Mixed | THC-scGF2dir | THC-scGF2 | fcCCSD |
| 16 | Ethene-Ethine | -3.94 | -2.84 | -1.244 |
| 17 | Benzene-$H_2O$ | — | -6.10 | -2.719 |
| 18 | Benzene-$NH_3$ | — | -5.24 | -1.793 |
| 19 | Benzene-HCN | — | -9.78 | -3.898 |

[1] T. Takatani, E. G. Hohenstein, M. Malagoli, M. S. Marshall, and C. D. Sherrill, Basis set consistent revision of the S22 test set of noncovalent interaction energies, J. Chem. Phys. **132**, 144104 (2010).

[2] L. A. Burns, M. S. Marshall, and C. D. Sherrill, Appointing silver and bronze standards for noncovalent interactions: A comparison of spin-component-scaled (SCS), explicitly correlated (F12), and specialized wavefunction approaches, J. Chem. Phys. **141**, 234111 (2014).
